# Supplementary material for: Occlusion-robust Stylization for Drawing-based 3D Animation
Source: arXiv:2508.00398 source file (2025-08-01)
Supplement: Supplementary file 1 [file X_suppl.tex]

\clearpage
\setcounter{page}{1}
\maketitlesupplementary

\section{Borader Impacts and Ethic Statements}
\label{sec:rationale}
Visual generative models present a range of ethical dilemmas, including the creation of unauthorized counterfeit content, potential privacy breaches, and challenges related to fairness.
Due to our reliance on the architecture of these models, our work inherently adopts these ethical vulnerabilities. 
Addressing these concerns is imperative and requires the establishment of comprehensive regulations and technical countermeasures.
It is the responsibility of researchers, including ourselves, to actively develop and apply these safeguards.
To promote transparency and encourage ethical use, we will release our source code along with detailed model and data specifications under a license that advocates lawful and responsible practices.
Furthermore, we are exploring advanced measures such as learning-based digital forensics and digital watermarking.
These efforts are part of a dedicated strategy to ethically navigate the complexities of visual generative models, ensuring their development serves the greater good.

\section{Limitation and Future work}
%
%human image animation system들은 reference 이미지를 주어진 target poses에 전달하는것을 목적으로 한다.
Human image animation systems transfer reference images to target poses. However, some frames in a target pose video may lack proper specification, leading to flicker or low fidelity in model predictions. Thus, integrating high-quality pose estimation is crucial.
%따라서 좋은 품질의 pose estimation을 함께 통합하는것이 중요하다.
%
%또 다른 한계로는 reference 와 target pose간의 human shape이 서로 너무 다른 경우 transfer된 결과가 어색하다.
Another limitation is that significant differences in body shape between the reference and target poses result in awkward transfers, such as transferring a skinny person to a large target pose. 
To achieve natural results, a system or module that aligns body shapes between poses is required. 
We plan to conduct further research to address these limitations in our future work.

\section{Details about Single-Step Drawing}

\section{Further qualitative results}
